# Supplementary material for: Emerging cooperation on the road by myopic local interactions
Source: arXiv:2208.03760 source file (2022-09-03)
Supplement: Supplementary file 1 [file Table.Ver_3101.All.Appendix.tex]

\documentclass{article}

\usepackage{standalone}
\usepackage{tikz}
\usepackage{amsmath, amssymb}
\usepackage{subcaption}
\usepackage{import}
\usepackage{fmtcount}
\usetikzlibrary{calc, patterns, intersections}

\begin{document}
	\begin{figure}[ht]
		\centering
		\begin{subfigure}[b]{0.27\textwidth}
			\centering
			\subimport{Ver.3101/}{Table.Ver_3101.Position_1}
			\caption{Position 1}
			\label{subfig:fg_3101_1}
		\end{subfigure}
		\hfill
		\begin{subfigure}[b]{0.69\textwidth}
			\centering
			\subimport{Ver.3101/}{Table.Ver_3101.Position_5}
			\caption{Position 5}
			\label{subfig:fg_3101_5}
		\end{subfigure}
		\caption{State machine(s) (\subref{subfig:fg_3101_1}) at position 1, (\subref{subfig:fg_3101_5}) at position 5.}
		\label{fig:fg_3101_1}
	\end{figure}
	\begin{figure}
		\centering
		\begin{subfigure}[b]{0.32\textwidth}
			\centering
			\subimport{Ver.3101/}{Table.Ver_3101.Position_2}
			\caption{Position 2}
			\label{subfig:fg_3101_2}
		\end{subfigure}
		\hfill
		\begin{subfigure}[b]{0.32\textwidth}
			\centering
			\subimport{Ver.3101/}{Table.Ver_3101.Position_3}
			\caption{Position 3}
			\label{subfig:fg_3101_3}
		\end{subfigure}
		\hfill
		\begin{subfigure}[b]{0.32\textwidth}
			\centering
			\subimport{Ver.3101/}{Table.Ver_3101.Position_4}
			\caption{Position 4}
			\label{subfig:fg_3101_4}
		\end{subfigure}
		\caption{State machine(s) (\subref{subfig:fg_3101_2}) at position 2, (\subref{subfig:fg_3101_3}) at position 3, (\subref{subfig:fg_3101_4}) at position 4.}
		\label{fig:fg_3101_2}
	\end{figure}
	\begin{figure}
		\centering
		\begin{subfigure}[b]{0.32\textwidth}
			\centering
			\subimport{Ver.3101/}{Table.Ver_3101.Position_6}
			\caption{Position 6}
			\label{subfig:fg_3101_6}
		\end{subfigure}
		\hfill
		\begin{subfigure}[b]{0.32\textwidth}
			\centering
			\subimport{Ver.3101/}{Table.Ver_3101.Position_7}
			\caption{Position 7}
			\label{subfig:fg_3101_7}
		\end{subfigure}
		\hfill
		\begin{subfigure}[b]{0.32\textwidth}
			\centering
			\subimport{Ver.3101/}{Table.Ver_3101.Position_8}
			\caption{Position 8}
			\label{subfig:fg_3101_8}
		\end{subfigure}
		\caption{State machine(s) (\subref{subfig:fg_3101_6}) at position 6, (\subref{subfig:fg_3101_7}) at position 7, (\subref{subfig:fg_3101_8}) at position 8.}
		\label{fig:fg_3101_3}
	\end{figure}
	\begin{figure}
		\centering
		\begin{subfigure}[b]{0.96\textwidth}
			\centering
			\subimport{Ver.3101/}{Table.Ver_3101.Position_9}
			\caption{Position 9}
			\label{subfig:fg_3101_9}
		\end{subfigure}
		\caption{State machine(s) (\subref{subfig:fg_3101_9}) at position 9.}
		\label{fig:fg_3101_4}
	\end{figure}
\end{document}
